# Supplementary material for: MEANTIME: Mixture of Attention Mechanisms with Multi-temporal Embeddings for Sequential Recommendation
Source: arXiv:2008.08273 source file (2020-08-21)
Supplement: Supplementary file 1 [file appendix_A.tex]

\label{app:fourier}
Paragraph.
