# Supplementary material for: MEANTIME: Mixture of Attention Mechanisms with Multi-temporal Embeddings for Sequential Recommendation
Source: arXiv:2008.08273 source file (2020-08-21)
Supplement: Supplementary file 2 [file appendix_B.tex]

\label{app:attnmaps}
